# Supplementary material for: Smooth-Trajectron++: Augmenting the Trajectron++ behaviour prediction model with smooth attention
Source: arXiv:2305.19678 source file (2023-06-02)
Supplement: Supplementary file 1 [file Appendix-tables.tex]

\section{Tables}
\label{appendix:tab}

\begin{table*}[h]
    \centering
    \caption{ROC curve at start (AUC)}
    \begin{tabularx}{\textwidth}{X | CC | CC | CC | CC | CC | CC} 
\toprule 
\multirow{2}{*}{\textbf{Dataset}} & \multicolumn{12}{c}{\textbf{Models}} \\
& \multicolumn{2}{c}{$T_{\beta_1}$}& \multicolumn{2}{c}{$T_{\beta_2}$}& \multicolumn{2}{c}{$T_{\beta_3}$}& \multicolumn{2}{c}{$T_{\beta_4}$}& \multicolumn{2}{c}{$T_{\beta_5}$}& \multicolumn{2}{c}{$T+$} \\
\midrule 
\emph{highD} (rest) & {\scriptsize $0.889^{\pm 0.036}$} & {\scriptsize $0.915^{\pm 0.018}$} & {\scriptsize $0.893^{\pm 0.039}$} & {\scriptsize $0.925^{\pm 0.040}$} & {\scriptsize $\underline{0.933}^{\pm 0.014}$} & {\scriptsize $\underline{0.949}^{\pm 0.007}$} & {\scriptsize $0.922^{\pm 0.025}$} & {\scriptsize $0.925^{\pm 0.023}$} & {\scriptsize $0.890^{\pm 0.027}$} & {\scriptsize $0.936^{\pm 0.018}$} & {\scriptsize $0.884^{\pm 0.055}$} & {\scriptsize $0.930^{\pm 0.011}$} \\ 
& {\scriptsize $0.472^{\hphantom{\pm 0.000}}$} & {\scriptsize $0.619^{\hphantom{\pm 0.000}}$} & {\scriptsize $0.506^{\hphantom{\pm 0.000}}$} & {\scriptsize $0.735^{\hphantom{\pm 0.000}}$} & {\scriptsize $0.473^{\hphantom{\pm 0.000}}$} & {\scriptsize $\underline{0.753}^{\hphantom{\pm 0.000}}$} & {\scriptsize $0.427^{\hphantom{\pm 0.000}}$} & {\scriptsize $0.689^{\hphantom{\pm 0.000}}$} & {\scriptsize $0.424^{\hphantom{\pm 0.000}}$} & {\scriptsize $0.612^{\hphantom{\pm 0.000}}$} & {\scriptsize $\underline{0.659}^{\hphantom{\pm 0.000}}$} & {\scriptsize $0.700^{\hphantom{\pm 0.000}}$} \\ 
\bottomrule
\end{tabularx}

    \label{tab:roc_start}
\end{table*}

\begin{table*}[h]
    \centering
    \caption{ROC curve at col (AUC)}
    \begin{tabularx}{\textwidth}{X | CC | CC | CC | CC | CC | CC} 
\toprule 
\multirow{2}{*}{\textbf{Dataset}} & \multicolumn{12}{c}{\textbf{Models}} \\
& \multicolumn{2}{c}{$T_{\beta_1}$}& \multicolumn{2}{c}{$T_{\beta_2}$}& \multicolumn{2}{c}{$T_{\beta_3}$}& \multicolumn{2}{c}{$T_{\beta_4}$}& \multicolumn{2}{c}{$T_{\beta_5}$}& \multicolumn{2}{c}{$T+$} \\
\midrule 
\emph{highD} (rest) & {\scriptsize $0.899^{\pm 0.028}$} & {\scriptsize $0.916^{\pm 0.015}$} & {\scriptsize $0.885^{\pm 0.050}$} & {\scriptsize $\underline{0.924}^{\pm 0.016}$} & {\scriptsize $\underline{0.919}^{\pm 0.014}$} & {\scriptsize $0.917^{\pm 0.020}$} & {\scriptsize $0.910^{\pm 0.013}$} & {\scriptsize $0.874^{\pm 0.031}$} & {\scriptsize $0.901^{\pm 0.028}$} & {\scriptsize $0.918^{\pm 0.012}$} & {\scriptsize $0.914^{\pm 0.010}$} & {\scriptsize $0.898^{\pm 0.038}$} \\ 
& {\scriptsize $0.653^{\hphantom{\pm 0.000}}$} & {\scriptsize $0.757^{\hphantom{\pm 0.000}}$} & {\scriptsize $0.653^{\hphantom{\pm 0.000}}$} & {\scriptsize $0.710^{\hphantom{\pm 0.000}}$} & {\scriptsize $0.725^{\hphantom{\pm 0.000}}$} & {\scriptsize $\underline{0.817}^{\hphantom{\pm 0.000}}$} & {\scriptsize $\underline{0.763}^{\hphantom{\pm 0.000}}$} & {\scriptsize $0.779^{\hphantom{\pm 0.000}}$} & {\scriptsize $0.624^{\hphantom{\pm 0.000}}$} & {\scriptsize $0.708^{\hphantom{\pm 0.000}}$} & {\scriptsize $0.633^{\hphantom{\pm 0.000}}$} & {\scriptsize $0.715^{\hphantom{\pm 0.000}}$} \\ 
\bottomrule
\end{tabularx}

    \label{tab:roc_col}
\end{table*}

\begin{table*}[h]
    \centering
    \caption{ADE at col}
    \begin{tabularx}{\textwidth}{X | CC | CC | CC | CC | CC | CC} 
\toprule 
\multirow{2}{*}{\textbf{Dataset}} & \multicolumn{12}{c}{\textbf{Models}} \\
& \multicolumn{2}{c}{$T_{\beta_1}$}& \multicolumn{2}{c}{$T_{\beta_2}$}& \multicolumn{2}{c}{$T_{\beta_3}$}& \multicolumn{2}{c}{$T_{\beta_4}$}& \multicolumn{2}{c}{$T_{\beta_5}$}& \multicolumn{2}{c}{$T+$} \\
\midrule 
\emph{highD} (rest) & {\scriptsize $4.861^{\pm 0.477}$} & {\scriptsize $4.198^{\pm 0.479}$} & {\scriptsize $5.895^{\pm 0.742}$} & {\scriptsize $5.121^{\pm 0.480}$} & {\scriptsize $4.590^{\pm 1.034}$} & {\scriptsize $\underline{4.120}^{\pm 0.159}$} & {\scriptsize $4.635^{\pm 0.409}$} & {\scriptsize $5.194^{\pm 1.244}$} & {\scriptsize $4.593^{\pm 0.387}$} & {\scriptsize $5.176^{\pm 0.624}$} & {\scriptsize $\underline{4.321}^{\pm 0.367}$} & {\scriptsize $6.214^{\pm 3.288}$} \\ 
& {\scriptsize $\underline{6.381}^{\hphantom{\pm 0.000}}$} & {\scriptsize $7.473^{\hphantom{\pm 0.000}}$} & {\scriptsize $7.295^{\hphantom{\pm 0.000}}$} & {\scriptsize $5.431^{\hphantom{\pm 0.000}}$} & {\scriptsize $6.434^{\hphantom{\pm 0.000}}$} & {\scriptsize $6.844^{\hphantom{\pm 0.000}}$} & {\scriptsize $7.319^{\hphantom{\pm 0.000}}$} & {\scriptsize $6.396^{\hphantom{\pm 0.000}}$} & {\scriptsize $6.825^{\hphantom{\pm 0.000}}$} & {\scriptsize $\underline{5.371}^{\hphantom{\pm 0.000}}$} & {\scriptsize $6.598^{\hphantom{\pm 0.000}}$} & {\scriptsize $5.743^{\hphantom{\pm 0.000}}$} \\ 
\bottomrule
\end{tabularx}

    \label{tab:ade_col}
\end{table*}

\begin{table*}[h]
    \centering
    \caption{FDE at col}
    \begin{tabularx}{\textwidth}{X | CC | CC | CC | CC | CC | CC} 
\toprule 
\multirow{2}{*}{\textbf{Dataset}} & \multicolumn{12}{c}{\textbf{Models}} \\
& \multicolumn{2}{c}{$T_{\beta_1}$}& \multicolumn{2}{c}{$T_{\beta_2}$}& \multicolumn{2}{c}{$T_{\beta_3}$}& \multicolumn{2}{c}{$T_{\beta_4}$}& \multicolumn{2}{c}{$T_{\beta_5}$}& \multicolumn{2}{c}{$T+$} \\
\midrule 
\emph{highD} (rest) & {\scriptsize $13.192^{\pm 1.884}$} & {\scriptsize $11.402^{\pm 1.697}$} & {\scriptsize $16.337^{\pm 2.082}$} & {\scriptsize $13.954^{\pm 1.107}$} & {\scriptsize $12.346^{\pm 3.286}$} & {\scriptsize $\underline{11.10}7^{\pm 0.464}$} & {\scriptsize $12.285^{\pm 1.593}$} & {\scriptsize $14.370^{\pm 3.614}$} & {\scriptsize $12.109^{\pm 1.024}$} & {\scriptsize $14.110^{\pm 1.482}$} & {\scriptsize $\underline{11.32}5^{\pm 1.023}$} & {\scriptsize $17.431^{\pm 10.003}$} \\ 
& {\scriptsize $\underline{16.56}2^{\hphantom{\pm 0.000}}$} & {\scriptsize $20.230^{\hphantom{\pm 0.000}}$} & {\scriptsize $19.131^{\hphantom{\pm 0.000}}$} & {\scriptsize $14.943^{\hphantom{\pm 0.000}}$} & {\scriptsize $17.325^{\hphantom{\pm 0.000}}$} & {\scriptsize $18.929^{\hphantom{\pm 0.000}}$} & {\scriptsize $19.694^{\hphantom{\pm 0.000}}$} & {\scriptsize $17.417^{\hphantom{\pm 0.000}}$} & {\scriptsize $18.364^{\hphantom{\pm 0.000}}$} & {\scriptsize $\underline{14.45}5^{\hphantom{\pm 0.000}}$} & {\scriptsize $17.230^{\hphantom{\pm 0.000}}$} & {\scriptsize $16.427^{\hphantom{\pm 0.000}}$} \\ 
\bottomrule
\end{tabularx}

    \label{tab:fde_col}
\end{table*}

\begin{table*}[h]
    \centering
    \caption{Brake at crit (TNR-PR)}
    \begin{tabularx}{\textwidth}{X | CC | CC | CC | CC | CC | CC} 
\toprule 
\multirow{2}{*}{\textbf{Dataset}} & \multicolumn{12}{c}{\textbf{Models}} \\
& \multicolumn{2}{c}{$T_{\beta_1}$}& \multicolumn{2}{c}{$T_{\beta_2}$}& \multicolumn{2}{c}{$T_{\beta_3}$}& \multicolumn{2}{c}{$T_{\beta_4}$}& \multicolumn{2}{c}{$T_{\beta_5}$}& \multicolumn{2}{c}{$T+$} \\
\midrule 
\emph{rounD} & {\scriptsize $\underline{1.000}^{\hphantom{\pm 0.000}}$} & {\scriptsize $\underline{1.000}^{\hphantom{\pm 0.000}}$} & {\scriptsize $\underline{1.000}^{\hphantom{\pm 0.000}}$} & {\scriptsize $\underline{1.000}^{\hphantom{\pm 0.000}}$} & {\scriptsize $\underline{1.000}^{\hphantom{\pm 0.000}}$} & {\scriptsize $\underline{1.000}^{\hphantom{\pm 0.000}}$} & {\scriptsize $\underline{1.000}^{\hphantom{\pm 0.000}}$} & {\scriptsize $\underline{1.000}^{\hphantom{\pm 0.000}}$} & {\scriptsize $\underline{1.000}^{\hphantom{\pm 0.000}}$} & {\scriptsize $\underline{1.000}^{\hphantom{\pm 0.000}}$} & {\scriptsize $\underline{1.000}^{\hphantom{\pm 0.000}}$} & {\scriptsize $\underline{1.000}^{\hphantom{\pm 0.000}}$} \\ 
& {\scriptsize $\underline{1.000}^{\hphantom{\pm 0.000}}$} & {\scriptsize $\underline{1.000}^{\hphantom{\pm 0.000}}$} & {\scriptsize $\underline{1.000}^{\hphantom{\pm 0.000}}$} & {\scriptsize $\underline{1.000}^{\hphantom{\pm 0.000}}$} & {\scriptsize $\underline{1.000}^{\hphantom{\pm 0.000}}$} & {\scriptsize $\underline{1.000}^{\hphantom{\pm 0.000}}$} & {\scriptsize $\underline{1.000}^{\hphantom{\pm 0.000}}$} & {\scriptsize $\underline{1.000}^{\hphantom{\pm 0.000}}$} & {\scriptsize $\underline{1.000}^{\hphantom{\pm 0.000}}$} & {\scriptsize $\underline{1.000}^{\hphantom{\pm 0.000}}$} & {\scriptsize $\underline{1.000}^{\hphantom{\pm 0.000}}$} & {\scriptsize $\underline{1.000}^{\hphantom{\pm 0.000}}$} \\ 
\midrule 
\emph{L-GAP} & {\scriptsize $\underline{0.599}^{\pm 0.350}$} & {\scriptsize $\underline{0.497}^{\pm 0.497}$} & {\scriptsize $\underline{0.599}^{\pm 0.350}$} & {\scriptsize $\underline{0.497}^{\pm 0.497}$} & {\scriptsize $\underline{0.599}^{\pm 0.350}$} & {\scriptsize $\underline{0.497}^{\pm 0.497}$} & {\scriptsize $\underline{0.599}^{\pm 0.350}$} & {\scriptsize $0.494^{\pm 0.494}$} & {\scriptsize $\underline{0.599}^{\pm 0.350}$} & {\scriptsize $0.494^{\pm 0.494}$} & {\scriptsize $\underline{0.599}^{\pm 0.350}$} & {\scriptsize $\underline{0.497}^{\pm 0.497}$} \\ 
& {\scriptsize $\underline{0.000}^{\hphantom{\pm 0.000}}$} & {\scriptsize $\underline{0.000}^{\hphantom{\pm 0.000}}$} & {\scriptsize $\underline{0.000}^{\hphantom{\pm 0.000}}$} & {\scriptsize $\underline{0.000}^{\hphantom{\pm 0.000}}$} & {\scriptsize $\underline{0.000}^{\hphantom{\pm 0.000}}$} & {\scriptsize $\underline{0.000}^{\hphantom{\pm 0.000}}$} & {\scriptsize $\underline{0.000}^{\hphantom{\pm 0.000}}$} & {\scriptsize $\underline{0.000}^{\hphantom{\pm 0.000}}$} & {\scriptsize $\underline{0.000}^{\hphantom{\pm 0.000}}$} & {\scriptsize $\underline{0.000}^{\hphantom{\pm 0.000}}$} & {\scriptsize $\underline{0.000}^{\hphantom{\pm 0.000}}$} & {\scriptsize $\underline{0.000}^{\hphantom{\pm 0.000}}$} \\ 
\bottomrule
\end{tabularx}

    \label{tab:brake_crit}
\end{table*}

\begin{table*}[h]
    \centering
    \caption{Accuracy at col}
    \begin{tabularx}{\textwidth}{X | CC | CC | CC | CC | CC | CC} 
\toprule 
\multirow{2}{*}{\textbf{Dataset}} & \multicolumn{12}{c}{\textbf{Models}} \\
& \multicolumn{2}{c}{$T_{\beta_1}$}& \multicolumn{2}{c}{$T_{\beta_2}$}& \multicolumn{2}{c}{$T_{\beta_3}$}& \multicolumn{2}{c}{$T_{\beta_4}$}& \multicolumn{2}{c}{$T_{\beta_5}$}& \multicolumn{2}{c}{$T+$} \\
\midrule 
\emph{highD} & {\scriptsize $0.915^{\pm 0.001}$} & {\scriptsize $0.927^{\pm 0.003}$} & {\scriptsize $0.911^{\pm 0.005}$} & {\scriptsize $\underline{0.929}^{\pm 0.009}$} & {\scriptsize $0.915^{\pm 0.007}$} & {\scriptsize $\underline{0.929}^{\pm 0.007}$} & {\scriptsize $0.919^{\pm 0.005}$} & {\scriptsize $0.927^{\pm 0.005}$} & {\scriptsize $\underline{0.920}^{\pm 0.002}$} & {\scriptsize $0.928^{\pm 0.006}$} & {\scriptsize $0.915^{\pm 0.002}$} & {\scriptsize $0.927^{\pm 0.003}$} \\ 
& {\scriptsize $0.901^{\hphantom{\pm 0.000}}$} & {\scriptsize $0.899^{\hphantom{\pm 0.000}}$} & {\scriptsize $0.901^{\hphantom{\pm 0.000}}$} & {\scriptsize $\underline{0.905}^{\hphantom{\pm 0.000}}$} & {\scriptsize $\underline{0.904}^{\hphantom{\pm 0.000}}$} & {\scriptsize $0.899^{\hphantom{\pm 0.000}}$} & {\scriptsize $0.902^{\hphantom{\pm 0.000}}$} & {\scriptsize $0.903^{\hphantom{\pm 0.000}}$} & {\scriptsize $0.902^{\hphantom{\pm 0.000}}$} & {\scriptsize $0.899^{\hphantom{\pm 0.000}}$} & {\scriptsize $0.901^{\hphantom{\pm 0.000}}$} & {\scriptsize $0.899^{\hphantom{\pm 0.000}}$} \\ 
\midrule 
\emph{highD} (rest) & {\scriptsize $0.836^{\pm 0.042}$} & {\scriptsize $0.844^{\pm 0.021}$} & {\scriptsize $0.842^{\pm 0.039}$} & {\scriptsize $\underline{0.858}^{\pm 0.032}$} & {\scriptsize $\underline{0.860}^{\pm 0.018}$} & {\scriptsize $0.839^{\pm 0.024}$} & {\scriptsize $0.844^{\pm 0.021}$} & {\scriptsize $0.803^{\pm 0.026}$} & {\scriptsize $0.851^{\pm 0.020}$} & {\scriptsize $0.846^{\pm 0.013}$} & {\scriptsize $0.858^{\pm 0.018}$} & {\scriptsize $0.835^{\pm 0.033}$} \\ 
& {\scriptsize $0.701^{\hphantom{\pm 0.000}}$} & {\scriptsize $0.704^{\hphantom{\pm 0.000}}$} & {\scriptsize $0.718^{\hphantom{\pm 0.000}}$} & {\scriptsize $0.704^{\hphantom{\pm 0.000}}$} & {\scriptsize $0.725^{\hphantom{\pm 0.000}}$} & {\scriptsize $\underline{0.773}^{\hphantom{\pm 0.000}}$} & {\scriptsize $\underline{0.732}^{\hphantom{\pm 0.000}}$} & {\scriptsize $0.734^{\hphantom{\pm 0.000}}$} & {\scriptsize $0.697^{\hphantom{\pm 0.000}}$} & {\scriptsize $0.665^{\hphantom{\pm 0.000}}$} & {\scriptsize $0.708^{\hphantom{\pm 0.000}}$} & {\scriptsize $0.708^{\hphantom{\pm 0.000}}$} \\ 
\midrule 
\emph{rounD} & {\scriptsize $\underline{0.952}^{\pm 0.015}$} & {\scriptsize $0.984^{\pm 0.005}$} & {\scriptsize $\underline{0.952}^{\pm 0.015}$} & {\scriptsize $\underline{0.991}^{\pm 0.005}$} & {\scriptsize $\underline{0.952}^{\pm 0.015}$} & {\scriptsize $0.984^{\pm 0.005}$} & {\scriptsize $\underline{0.952}^{\pm 0.015}$} & {\scriptsize $\underline{0.991}^{\pm 0.005}$} & {\scriptsize $\underline{0.952}^{\pm 0.015}$} & {\scriptsize $0.987^{\hphantom{\pm 0.000}}$} & {\scriptsize $\underline{0.952}^{\pm 0.015}$} & {\scriptsize $0.987^{\hphantom{\pm 0.000}}$} \\ 
& {\scriptsize $\underline{0.890}^{\hphantom{\pm 0.000}}$} & {\scriptsize $0.935^{\hphantom{\pm 0.000}}$} & {\scriptsize $\underline{0.890}^{\hphantom{\pm 0.000}}$} & {\scriptsize $0.948^{\hphantom{\pm 0.000}}$} & {\scriptsize $\underline{0.890}^{\hphantom{\pm 0.000}}$} & {\scriptsize $\underline{0.974}^{\hphantom{\pm 0.000}}$} & {\scriptsize $\underline{0.890}^{\hphantom{\pm 0.000}}$} & {\scriptsize $0.935^{\hphantom{\pm 0.000}}$} & {\scriptsize $\underline{0.890}^{\hphantom{\pm 0.000}}$} & {\scriptsize $0.948^{\hphantom{\pm 0.000}}$} & {\scriptsize $\underline{0.890}^{\hphantom{\pm 0.000}}$} & {\scriptsize $0.935^{\hphantom{\pm 0.000}}$} \\ 
\midrule 
\emph{L-GAP} & {\scriptsize $\underline{0.889}^{\pm 0.016}$} & {\scriptsize $0.991^{\pm 0.003}$} & {\scriptsize $\underline{0.889}^{\pm 0.016}$} & {\scriptsize $0.986^{\pm 0.005}$} & {\scriptsize $\underline{0.889}^{\pm 0.016}$} & {\scriptsize $0.987^{\pm 0.008}$} & {\scriptsize $\underline{0.889}^{\pm 0.016}$} & {\scriptsize $0.986^{\pm 0.007}$} & {\scriptsize $\underline{0.889}^{\pm 0.016}$} & {\scriptsize $\underline{0.992}^{\pm 0.007}$} & {\scriptsize $\underline{0.889}^{\pm 0.016}$} & {\scriptsize $0.984^{\pm 0.007}$} \\ 
& {\scriptsize $\underline{0.590}^{\hphantom{\pm 0.000}}$} & {\scriptsize $0.904^{\hphantom{\pm 0.000}}$} & {\scriptsize $\underline{0.590}^{\hphantom{\pm 0.000}}$} & {\scriptsize $\underline{0.910}^{\hphantom{\pm 0.000}}$} & {\scriptsize $\underline{0.590}^{\hphantom{\pm 0.000}}$} & {\scriptsize $0.904^{\hphantom{\pm 0.000}}$} & {\scriptsize $\underline{0.590}^{\hphantom{\pm 0.000}}$} & {\scriptsize $\underline{0.910}^{\hphantom{\pm 0.000}}$} & {\scriptsize $\underline{0.590}^{\hphantom{\pm 0.000}}$} & {\scriptsize $0.904^{\hphantom{\pm 0.000}}$} & {\scriptsize $\underline{0.590}^{\hphantom{\pm 0.000}}$} & {\scriptsize $\underline{0.910}^{\hphantom{\pm 0.000}}$} \\ 
\bottomrule
\end{tabularx}

    \label{tab:acc_col}
\end{table*}

\begin{table*}[h]
    \centering
    \caption{Accuracy at start}
    \begin{tabularx}{\textwidth}{X | CC | CC | CC | CC | CC | CC} 
\toprule 
\multirow{2}{*}{\textbf{Dataset}} & \multicolumn{12}{c}{\textbf{Models}} \\
& \multicolumn{2}{c}{$T_{\beta_1}$}& \multicolumn{2}{c}{$T_{\beta_2}$}& \multicolumn{2}{c}{$T_{\beta_3}$}& \multicolumn{2}{c}{$T_{\beta_4}$}& \multicolumn{2}{c}{$T_{\beta_5}$}& \multicolumn{2}{c}{$T+$} \\
\midrule 
\emph{highD} & {\scriptsize $0.871^{\pm 0.016}$} & {\scriptsize $0.885^{\pm 0.006}$} & {\scriptsize $0.874^{\pm 0.010}$} & {\scriptsize $0.887^{\pm 0.007}$} & {\scriptsize $\underline{0.881}^{\pm 0.010}$} & {\scriptsize $0.883^{\pm 0.015}$} & {\scriptsize $0.876^{\pm 0.006}$} & {\scriptsize $0.891^{\pm 0.007}$} & {\scriptsize $0.879^{\pm 0.007}$} & {\scriptsize $0.884^{\pm 0.010}$} & {\scriptsize $0.876^{\pm 0.013}$} & {\scriptsize $\underline{0.894}^{\pm 0.006}$} \\ 
& {\scriptsize $0.833^{\hphantom{\pm 0.000}}$} & {\scriptsize $0.837^{\hphantom{\pm 0.000}}$} & {\scriptsize $0.836^{\hphantom{\pm 0.000}}$} & {\scriptsize $0.837^{\hphantom{\pm 0.000}}$} & {\scriptsize $0.833^{\hphantom{\pm 0.000}}$} & {\scriptsize $0.837^{\hphantom{\pm 0.000}}$} & {\scriptsize $0.833^{\hphantom{\pm 0.000}}$} & {\scriptsize $0.837^{\hphantom{\pm 0.000}}$} & {\scriptsize $0.838^{\hphantom{\pm 0.000}}$} & {\scriptsize $\underline{0.848}^{\hphantom{\pm 0.000}}$} & {\scriptsize $\underline{0.842}^{\hphantom{\pm 0.000}}$} & {\scriptsize $0.840^{\hphantom{\pm 0.000}}$} \\ 
\midrule 
\emph{highD} (rest) & {\scriptsize $0.826^{\pm 0.047}$} & {\scriptsize $0.870^{\pm 0.010}$} & {\scriptsize $0.831^{\pm 0.041}$} & {\scriptsize $0.880^{\pm 0.037}$} & {\scriptsize $\underline{0.874}^{\pm 0.017}$} & {\scriptsize $\underline{0.904}^{\pm 0.015}$} & {\scriptsize $0.873^{\pm 0.034}$} & {\scriptsize $0.893^{\pm 0.012}$} & {\scriptsize $0.852^{\pm 0.036}$} & {\scriptsize $0.899^{\pm 0.031}$} & {\scriptsize $0.841^{\pm 0.056}$} & {\scriptsize $0.889^{\pm 0.019}$} \\ 
& {\scriptsize $0.604^{\hphantom{\pm 0.000}}$} & {\scriptsize $0.684^{\hphantom{\pm 0.000}}$} & {\scriptsize $0.581^{\hphantom{\pm 0.000}}$} & {\scriptsize $0.711^{\hphantom{\pm 0.000}}$} & {\scriptsize $0.604^{\hphantom{\pm 0.000}}$} & {\scriptsize $\underline{0.729}^{\hphantom{\pm 0.000}}$} & {\scriptsize $0.590^{\hphantom{\pm 0.000}}$} & {\scriptsize $0.703^{\hphantom{\pm 0.000}}$} & {\scriptsize $0.588^{\hphantom{\pm 0.000}}$} & {\scriptsize $0.695^{\hphantom{\pm 0.000}}$} & {\scriptsize $\underline{0.661}^{\hphantom{\pm 0.000}}$} & {\scriptsize $0.679^{\hphantom{\pm 0.000}}$} \\ 
\midrule 
\emph{rounD} & {\scriptsize $\underline{0.970}^{\pm 0.004}$} & {\scriptsize $0.983^{\pm 0.008}$} & {\scriptsize $0.969^{\pm 0.009}$} & {\scriptsize $0.981^{\pm 0.005}$} & {\scriptsize $0.964^{\pm 0.008}$} & {\scriptsize $\underline{0.984}^{\pm 0.007}$} & {\scriptsize $\underline{0.970}^{\pm 0.001}$} & {\scriptsize $0.982^{\pm 0.004}$} & {\scriptsize $0.969^{\pm 0.003}$} & {\scriptsize $0.982^{\pm 0.002}$} & {\scriptsize $0.967^{\pm 0.006}$} & {\scriptsize $0.978^{\pm 0.006}$} \\ 
& {\scriptsize $0.852^{\hphantom{\pm 0.000}}$} & {\scriptsize $0.917^{\hphantom{\pm 0.000}}$} & {\scriptsize $\underline{0.856}^{\hphantom{\pm 0.000}}$} & {\scriptsize $\underline{0.921}^{\hphantom{\pm 0.000}}$} & {\scriptsize $0.843^{\hphantom{\pm 0.000}}$} & {\scriptsize $\underline{0.921}^{\hphantom{\pm 0.000}}$} & {\scriptsize $0.836^{\hphantom{\pm 0.000}}$} & {\scriptsize $0.913^{\hphantom{\pm 0.000}}$} & {\scriptsize $0.852^{\hphantom{\pm 0.000}}$} & {\scriptsize $0.909^{\hphantom{\pm 0.000}}$} & {\scriptsize $0.839^{\hphantom{\pm 0.000}}$} & {\scriptsize $0.917^{\hphantom{\pm 0.000}}$} \\ 
\midrule 
\emph{L-GAP} & {\scriptsize $\underline{0.688}^{\pm 0.022}$} & {\scriptsize $0.988^{\pm 0.006}$} & {\scriptsize $\underline{0.688}^{\pm 0.022}$} & {\scriptsize $0.985^{\pm 0.007}$} & {\scriptsize $\underline{0.688}^{\pm 0.022}$} & {\scriptsize $0.985^{\pm 0.010}$} & {\scriptsize $\underline{0.688}^{\pm 0.022}$} & {\scriptsize $0.988^{\pm 0.006}$} & {\scriptsize $\underline{0.688}^{\pm 0.022}$} & {\scriptsize $0.983^{\pm 0.011}$} & {\scriptsize $\underline{0.688}^{\pm 0.022}$} & {\scriptsize $\underline{0.989}^{\pm 0.005}$} \\ 
& {\scriptsize $\underline{0.505}^{\hphantom{\pm 0.000}}$} & {\scriptsize $\underline{0.920}^{\hphantom{\pm 0.000}}$} & {\scriptsize $\underline{0.505}^{\hphantom{\pm 0.000}}$} & {\scriptsize $0.914^{\hphantom{\pm 0.000}}$} & {\scriptsize $\underline{0.505}^{\hphantom{\pm 0.000}}$} & {\scriptsize $0.914^{\hphantom{\pm 0.000}}$} & {\scriptsize $\underline{0.505}^{\hphantom{\pm 0.000}}$} & {\scriptsize $0.907^{\hphantom{\pm 0.000}}$} & {\scriptsize $\underline{0.505}^{\hphantom{\pm 0.000}}$} & {\scriptsize $0.907^{\hphantom{\pm 0.000}}$} & {\scriptsize $\underline{0.505}^{\hphantom{\pm 0.000}}$} & {\scriptsize $\underline{0.920}^{\hphantom{\pm 0.000}}$} \\ 
\bottomrule
\end{tabularx}

    \label{tab:acc_start}
\end{table*}
